# Supplementary material for: NeoMem: Hardware/Software Co-Design for CXL-Native Memory Tiering
Source: arXiv:2403.18702 source file (2024-09-11)
Supplement: Supplementary file 1 [file AE_appendix.tex]

\appendix
\section{Artifact Appendix}

%%%%%%%%%%%%%%%%%%%%%%%%%%%%%%%%%%%%%%%%%%%%%%%%%%%%%%%%%%%%%%%%%%%%%
\subsection{Abstract}

% {\em Obligatory. Summarize your artifacts (including algorithms, models, data sets, software and hardware) 
% and how they help to reproduce the key results from your paper.}

The implementation of NeoMem consists of the SystemVerilog code for the NeoProf hardware, the Linux kernel with added drivers for NeoMem, and benchmarking scripts. The source code for NeoMem is available at ~\url{https://github.com/PKUZHOU/NeoMem-MICRO-2024}.

\subsection{Artifact check-list (meta-information)}

% {\em Obligatory. Use just a few informal keywords in all fields applicable to your artifacts
% and remove the rest. This information is needed to find appropriate reviewers and gradually 
% unify artifact meta information in Digital Libraries.}

{\small
\begin{itemize}
  % \item {\bf Algorithm: }
  % \item {\bf Program: }
  % \item {\bf Compilation: }
  % \item {\bf Transformations: }
  % \item {\bf Binary: }
  % \item {\bf Model: }
  % \item {\bf Data set: }
  % \item {\bf Run-time environment: }
  \item {\bf Hardware: }An Intel Agilex-7 I series FPGA and a single socket Xeon 4th 6430 CPU.
  % \item {\bf Run-time state: }
  % \item {\bf Execution: }
  % \item {\bf Metrics: }
  \item {\bf Output: }Performance and profiling statistics of the benchmarks.
  % \item {\bf Experiments: }
  % \item {\bf How much disk space required (approximately)?: }
  \item {\bf How much time is needed to prepare workflow (approximately)?: }1 hour.
  \item {\bf How much time is needed to complete experiments (approximately)?: }8 hours.
  \item {\bf Publicly available?: }Yes.
  % \item {\bf Code licenses (if publicly available)?: GPLv2}
  % \item {\bf Data licenses (if publicly available)?: }
  % \item {\bf Workflow automation framework used?: }
  % \item {\bf Archived (provide DOI)?: }
\end{itemize}
}

%%%%%%%%%%%%%%%%%%%%%%%%%%%%%%%%%%%%%%%%%%%%%%%%%%%%%%%%%%%%%%%%%%%%%
\subsection{Description}

\subsubsection{How to access}
We offer remote access to our machine. To connect, please use the following command:
\begin{lstlisting}
ssh -p 6000 micro24@47.104.104.142
\end{lstlisting}
The password is \texttt{\textbf{neomemae}}.
% {\em Obligatory}

% \subsubsection{Hardware dependencies}

% \subsubsection{Software dependencies}

% \subsubsection{Data sets}

% \subsubsection{Models}

%%%%%%%%%%%%%%%%%%%%%%%%%%%%%%%%%%%%%%%%%%%%%%%%%%%%%%%%%%%%%%%%%%%%%
\subsection{Installation}
% {\em Obligatory}
To install the NeoMem system on your own, run:
\begin{lstlisting}
git clone git@github.com:PKUZHOU/NeoMem-MICRO-2024.git
cd NeoMem-MICRO-2024
git submodule update --init
\end{lstlisting}

Next, install the provided kernel on your machine, compile the hardware code using Quartus 22.3, and program the FPGA with the generated bitstream. After that, run the benchmarking scripts. For more details, visit~\url{https://github.com/PKUZHOU/NeoMem-MICRO-2024}.  

%%%%%%%%%%%%%%%%%%%%%%%%%%%%%%%%%%%%%%%%%%%%%%%%%%%%%%%%%%%%%%%%%%%%%
\subsection{Experiment workflow}
% First, log in to our machine using the provided remote access.
% \begin{lstlisting}
% ssh -p 6000 micro24@47.104.104.142
% passwd: neomemae
% \end{lstlisting}

Then, run:
\begin{lstlisting}
cd /home/micro24/NeoMem_AE
python run_all.py
\end{lstlisting}

This script will run experiments for Figure~\ref{fig:performance_overview} and Figure~\ref{fig:overall_analysis}, which takes approximately 6 hours. 
We recommend using a tool like \texttt{tmux} (already installed on our machine) to run the script in the background.
The output will be saved in \texttt{output/experiment\_output}.

Then, run:
\begin{lstlisting}
python run_convergence_curve.py
\end{lstlisting}

This script will run experiments for Figure~\ref{fig:motivation_converge}, which takes approximately 2 hours. The output will be saved in \texttt{output/gups\_convergence\_analysis}.

After completing the above scripts, run:
\begin{lstlisting}
python parse_result.py
\end{lstlisting}

This script generates visualizations of the experiment results. You can view the visualized results in \texttt{output/fig\_output}.

%%%%%%%%%%%%%%%%%%%%%%%%%%%%%%%%%%%%%%%%%%%%%%%%%%%%%%%%%%%%%%%%%%%%%
\subsection{Evaluation and Expected Results}

The figures located in the \texttt{output/fig\_output} directory will accurately reproduce the results depicted in Figure~\ref{fig:performance_overview}, Figure~\ref{fig:overall_analysis}, and Figure~\ref{fig:motivation_converge}. You will see that NeoMem demonstrates superior performance over all baseline systems, consistently across every benchmark. Additionally, Figure 13  is presented as a collection of sub-figures for convenience of drawing. 

%%%%%%%%%%%%%%%%%%%%%%%%%%%%%%%%%%%%%%%%%%%%%%%%%%%%%%%%%%%%%%%%%%%%%
% \subsection{Experiment customization}

%%%%%%%%%%%%%%%%%%%%%%%%%%%%%%%%%%%%%%%%%%%%%%%%%%%%%%%%%%%%%%%%%%%%%
% \subsection{Notes}

%%%%%%%%%%%%%%%%%%%%%%%%%%%%%%%%%%%%%%%%%%%%%%%%%%%%%%%%%%%%%%%%%%%%%
% \subsection{Methodology}

% Submission, reviewing and badging methodology:

% \begin{itemize}
%   \item \url{https://www.acm.org/publications/policies/artifact-review-and-badging-current}
%   \item \url{https://cTuning.org/ae}
% \end{itemize}

%%%%%%%%%%%%%%%%%%%%%%%%%%%%%%%%%%%%%%%%%%%%%%%%%%%%
% When adding this appendix to your paper, 
% please remove below part
%%%%%%%%%%%%%%%%%%%%%%%%%%%%%%%%%%%%%%%%%%%%%%%%%%%%
